# Supplementary material for: MAGDiff: Covariate Data Set Shift Detection via Activation Graphs of Deep Neural Networks
Source: arXiv:2305.13271 source file (2024-05-12)
Supplement: Supplementary file 1 [file full_table_MNIST_CIFAR10.tex]

\setlength{\tabcolsep}{0.4em}
\begin{tabular}{lcr c rrrrrrr c ccccccc}
 & & & & \multicolumn{7}{c}{MNIST}& & \multicolumn{7}{c}{CIFAR10}\\
\hhline{~~~~-------~-------}
 \multirow{2}{*}{Shift} &  \multirow{2}{*}{Int.} & \multirow{2}{*}{Feat.}  & &\multicolumn{7}{c}{Sample size} & &\multicolumn{7}{c}{Sample size}\\
\hhline{~~~~-------~-------}
 &  & &  & 10 & 20 & 50 & 100 & 200 & 500 & 1000 & &  10 & 20 & 50 & 100 & 200 & 500 & 1000  \\
\hhline{===~=======~=======}
\multirow{6}{*}{GN}  & \multirow{2}{*}{II} & \texttt{MD} &  &  $ 2.7 \pm 0.8 $ & $ 7.7 \pm 1.3 $ & $ 11.2 \pm 1.6 $ & $ 29.3 \pm 2.3 $ & $ 55.9 \pm 2.5 $ & $ 94.7 \pm 1.1 $ & $ 99.9 \pm 0.1 $ & &  $ 1.8 \pm 0.7 $ & $ 5.3 \pm 1.1 $ & $ 16.7 \pm 1.9 $ & $ 47.0 \pm 2.5 $ & $ 86.9 \pm 1.7 $ & $ 100.0 - 0.0 $ & $ 100.0 - 0.0 $ \\
 & & CV &  &  $ 0.0 + 0.2 $ & $ 0.1 \pm 0.1 $ & $ 0.0 + 0.2 $ & $ 0.1 \pm 0.1 $ & $ 0.3 \pm 0.3 $ & $ 1.5 \pm 0.6 $ & $ 6.1 \pm 1.2 $ & &  $ 2.3 \pm 0.8 $ & $ 4.5 \pm 1.1 $ & $ 6.9 \pm 1.3 $ & $ 19.1 \pm 2.0 $ & $ 38.3 \pm 2.5 $ & $ 88.3 \pm 1.6 $ & $ 99.9 \pm 0.1 $ \\
  & \multirow{2}{*}{IV} & \texttt{MD} &  &  $ 8.6 \pm 1.4 $ & $ 26.1 \pm 2.2 $ & $ 60.9 \pm 2.5 $ & $ 93.3 \pm 1.3 $ & $ 100.0 - 0.0 $ & $ 100.0 - 0.0 $ & $ 100.0 - 0.0 $ & &  $ 2.5 \pm 0.8 $ & $ 11.1 \pm 1.6 $ & $ 36.7 \pm 2.4 $ & $ 81.1 \pm 2.0 $ & $ 99.3 \pm 0.4 $ & $ 100.0 - 0.0 $ & $ 100.0 - 0.0 $ \\
 & & CV &  &  $ 0.1 \pm 0.2 $ & $ 1.0 \pm 0.5 $ & $ 3.8 \pm 1.0 $ & $ 17.6 \pm 1.9 $ & $ 58.4 \pm 2.5 $ & $ 99.3 \pm 0.4 $ & $ 100.0 - 0.0 $ & &  $ 2.5 \pm 0.8 $ & $ 6.7 \pm 1.3 $ & $ 11.7 \pm 1.6 $ & $ 29.9 \pm 2.3 $ & $ 63.4 \pm 2.4 $ & $ 99.3 \pm 0.4 $ & $ 100.0 - 0.0 $ \\
   & \multirow{2}{*}{VI} & \texttt{MD} &  &  $ 16.5 \pm 1.9 $ & $ 54.2 \pm 2.5 $ & $ 93.5 \pm 1.3 $ & $ 100.0 - 0.0 $ & $ 100.0 - 0.0 $ & $ 100.0 - 0.0 $ & $ 100.0 - 0.0 $ & &  $ 2.7 \pm 0.8 $ & $ 14.7 \pm 1.8 $ & $ 49.2 \pm 2.5 $ & $ 91.2 \pm 1.4 $ & $ 99.9 \pm 0.1 $ & $ 100.0 - 0.0 $ & $ 100.0 - 0.0 $ \\
 & & CV &  &  $ 3.7 \pm 1.0 $ & $ 20.4 \pm 2.0 $ & $ 65.6 \pm 2.4 $ & $ 98.9 \pm 0.5 $ & $ 100.0 - 0.0 $ & $ 100.0 - 0.0 $ & $ 100.0 - 0.0 $ & &  $ 2.7 \pm 0.8 $ & $ 7.3 \pm 1.3 $ & $ 14.2 \pm 1.8 $ & $ 37.5 \pm 2.5 $ & $ 77.3 \pm 2.1 $ & $ 99.9 \pm 0.2 $ & $ 100.0 - 0.0 $ \\
\hhline{---~-------~-------}
\multirow{6}{*}{IS}  & \multirow{2}{*}{II} & \texttt{MD} &  &  3.12 & 3.16 & 2.18 & 1.89 & 1.85 & 1.89 & 1.85 & &  3.12 & 3.16 & 2.18 & 1.89 & 1.85 & 1.89 & 1.85 \\
 & & CV &  &  3.12 & 3.16 & 2.18 & 1.89 & 1.85 & 1.89 & 1.85 & &  3.12 & 3.16 & 2.18 & 1.89 & 1.85 & 1.89 & 1.85 \\
  & \multirow{2}{*}{IV} & \texttt{MD} &  &  3.12 & 3.16 & 2.18 & 1.89 & 1.85 & 1.89 & 1.85 & &  3.12 & 3.16 & 2.18 & 1.89 & 1.85 & 1.89 & 1.85 \\
 & & CV &  &  3.12 & 3.16 & 2.18 & 1.89 & 1.85 & 1.89 & 1.85 & &  3.12 & 3.16 & 2.18 & 1.89 & 1.85 & 1.89 & 1.85 \\
   & \multirow{2}{*}{VI} & \texttt{MD} &  &  3.12 & 3.16 & 2.18 & 1.89 & 1.85 & 1.89 & 1.85 & &  3.12 & 3.16 & 2.18 & 1.89 & 1.85 & 1.89 & 1.85 \\
 & & CV &  &  3.12 & 3.16 & 2.18 & 1.89 & 1.85 & 1.89 & 1.85 & &  3.12 & 3.16 & 2.18 & 1.89 & 1.85 & 1.89 & 1.85 \\
\hline
\end{tabular}
